# Supplementary material for: Unified Weak-to-Strong Coupling Transitions and Radiation Interference Induced by Vertical-Symmetry Breaking in Photonic Crystal Slabs
Source: arXiv:1905.03868 source file (2026-06-22)
Supplement: Supplementary file 1 [file SI.pdf]

# Supplemental Information: Realization of Bound state In the Continuum induced by vertical symmetry breaking in photonic lattice

R. Mermet-Lyaudoz<sup>1</sup>, F. Dubois<sup>1</sup>, N-V. Hoang<sup>1</sup>, E. Drouard<sup>1</sup>, L. Berguiga<sup>2</sup>, C. Seassal<sup>1</sup>, X. Letartre<sup>1</sup>, P. Viktorovitch<sup>1</sup>, and H. S. Nguyen<sup>1\*</sup>  
<sup>1</sup> *Université de Lyon, Institut des Nanotechnologies de Lyon, INL/CNRS, Ecole Centrale de Lyon, 36 avenue Guy de Collongue, 69130 Ecully, France and*  
<sup>2</sup> *Université de Lyon, Institut des Nanotechnologies de Lyon, INL/CNRS, INSA-Lyon, 7 avenue Jean Capelle, 69621 Villeurbanne, France*

## I. SYMMETRY-BREAKING BIC IN P-POLARIZED ( $H_y$ FIELD)

Figure 1 presents the experimental results [Fig.1.(a)] and numerical simulation [Fig.1.(b)] of the angle-resolved reflectivity in p-polarized (i.e.  $H_y$  field). The experiments are performed on the same sample as presented in the main text. Similar symmetry-breaking BIC as the one in s-polarization, is clearly evidenced: i) Far from the anti-crossing point, the two modes are either even-like (point M and S) or odd-like (point Q and P); ii) At the anti-crossing point, there is a balanced mixing between odd and even (point N and R); iii) The symmetry-breaking BIC (vanishing of the Fano resonance) is observed in the vicinity of the anticrossing point, in the lower branch.

We note that in the case of p-polarized, the linewidths of uncoupled modes are very different:  $\gamma_e \gg \gamma_o$  [see Fig.1(a)], thus the angular position  $\theta_{BIC}$  of the symmetry-breaking BIC is greatly shifted with respect to  $\theta_{AC}$  of the anticrossing point with  $|\theta_{AC} - \theta_{BIC}| = 2^\circ$  (see eq. (2) in the main text). This is very different from the case of s-polarized in which  $\gamma_e \approx \gamma_o$ , leading to  $|\theta_{AC} - \theta_{BIC}| = 0.5^\circ$ .

## II. ROBUSTNESS AND TUNABILITY OF SYMMETRY-BREAKING BIC

As discussed in the main text, the robustness of the symmetry-breaking BIC is tested by performing angle-resolved reflectivity for different etching coefficient  $\epsilon$  while keeping fixed all other parameters ( $a = 354$  nm,  $d = 160$  nm,  $h = 130$  nm). The results are presented in Fig.2, with spectral resolution corresponding to quality factor  $Q = 10^5$ . It is shown that: i) Loss-exchange always occurs, the upper/lower branch is broaden/narrowed when getting close to the anticrossing point; ii) The vanishing of the Fano resonance in the lower branch is only observed for  $\epsilon < 65\%$ . It shows that the symmetry-breaking BIC is rather a quasi-BIC than a BIC. This is due to the fact that the phase-shift  $\psi$  between two resonances are not really zero. Nevertheless, by changing  $\epsilon$ , we probably

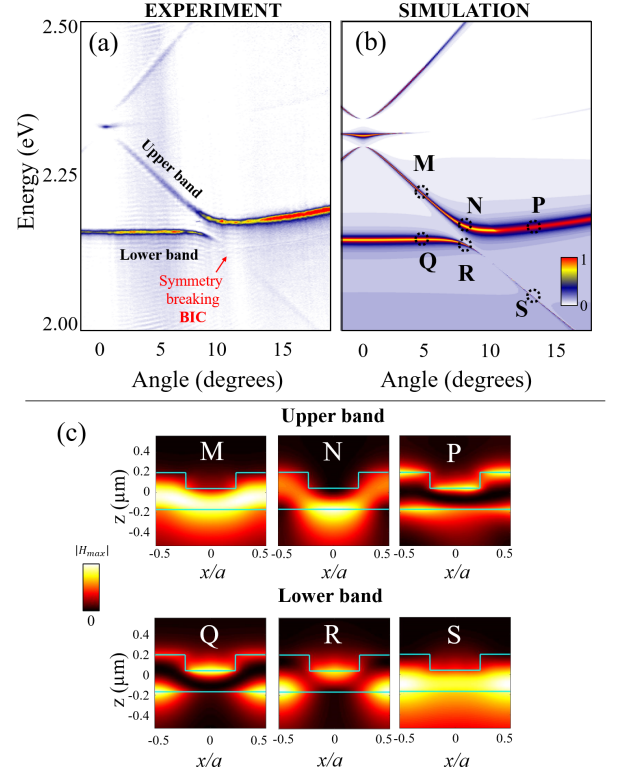

FIG. 1. (a) Experimental measurement and (b) Numerical simulations of the p-polarized angle-resolved reflectivity. (c) Distribution of the magnetic field intensity  $|H(x, y = 0, z)|$  on different points of the upper and lower band of (b).

manage to obtain an authentic BIC, as the case for an accidental BIC obtained through parameter tuning.

It is interesting to note that when changing the etching coefficient  $\epsilon$ , the angular position  $\theta_{BIC}$  of symmetry-breaking BIC is almost unchanged (see Fig.2). Otherwise, it is shown in the main text that changing the aspect ratio  $d/a$  can drag  $\theta_{BIC}$  of the symmetry-breaking BIC within the Fourier plan. As a consequence,  $\epsilon$  and  $d/a$  are two parameters that can be used independently to create and locate a symmetry-breaking BIC: i)  $\epsilon$  for optimizing the quality factor of the quasi-BIC; ii)  $d/a$  for modifying its angular position.

\* hai-son.nguyen@ec-lyon.fr

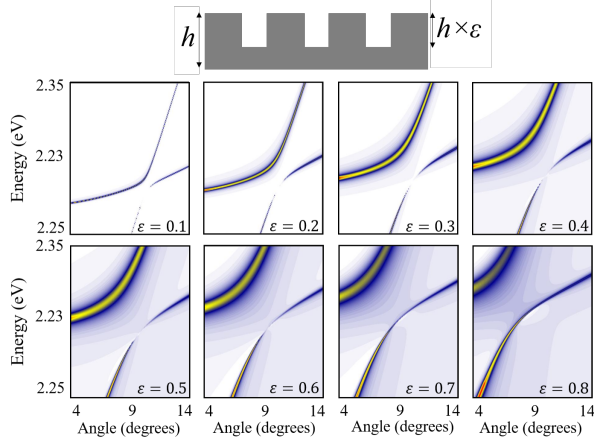

FIG. 2. Evolution of the s-polarized angle-resolved reflectivity depending on the etching depth. The inset depicts the scheme of the structure exhibiting the varying  $\epsilon$ .

### III. NUMERICAL ESTIMATION OF THE COUPLING STRENGTH

The coupling strength  $\kappa$  between even-like and odd-like modes in eq.(1) of the main text can be estimated numerically via an perturbation approach based on coupled mode theory, given by [1, 2]:

$$|\kappa| = \frac{E_C}{2} \frac{\left| \int_V \vec{\mathcal{E}}_e^*(\vec{r}) \cdot \vec{\mathcal{E}}_o(\vec{r}) \cdot \Delta\epsilon(\vec{r}) dV \right|}{\sqrt{\int_V |\vec{\mathcal{E}}_e(\vec{r})|^2 \cdot \epsilon(\vec{r}) dV} \sqrt{\int_V |\vec{\mathcal{E}}_o(\vec{r})|^2 \epsilon(\vec{r}) dV}}$$

where  $\vec{\mathcal{E}}_{e(o)}(\vec{r})$  is the electric field of the even(odd) mode of the perfectly symmetric structure [see Fig.3(b)];  $\epsilon(\vec{r})$  is the permittivity of the perfect symmetric structure [see Fig.3(a)]; and  $\Delta\epsilon(\vec{r})$  is the modification of the permittivity from its initial function  $\epsilon(\vec{r})$  when considering the structure of broken vertical symmetry [see Fig.3(b)].

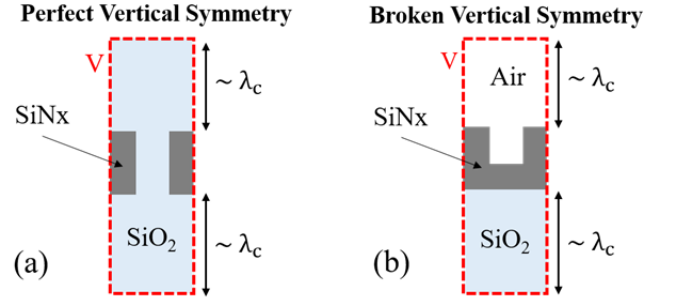

FIG. 3. (a,b) Sketch of the structure exhibiting (a) Full vertical symmetry and (b) Broken vertical symmetry.

This coupling strength needs to be evaluated at the phase matching condition (crossing point of the two

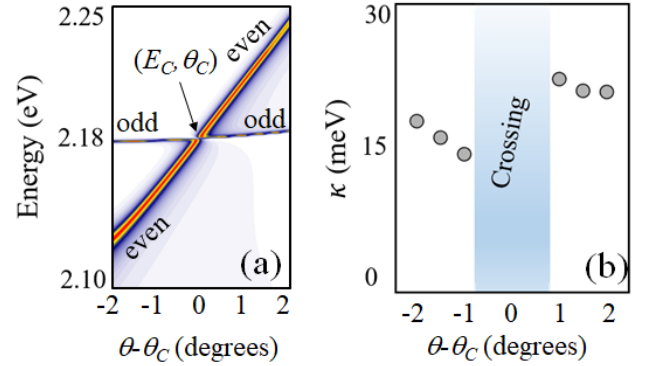

FIG. 4. (a) Simulation of the s-polarized angle-resolved reflectivity for the perfectly vertical symmetric structure [Fig.3(a)]. (b) Numerical estimation the coupling strength  $\kappa$ .

uncoupled dispersions) of energy  $E_C = 2.18$  eV [see Fig.4(a)]. However, the electric field  $\vec{\mathcal{E}}_{e(o)}(\vec{r})$  can not be properly extracted at the crossing point since there will be overlap between the two modes. Thus we estimate  $\kappa$  using  $\vec{\mathcal{E}}_{e(o)}(\vec{r})$  computed in the vicinity of the crossing point. For the integral, we consider that the unit cell  $V$  extends to one wavelength  $\lambda_C = \frac{2\pi\hbar c}{E_C}$  below and above the slab [see Fig.2(a) and (b)]. The numerical results are depicted in Fig.4(b), showing  $\kappa$  in the range of 20 meV. This is quite close to the value 18 meV that we obtain by fitting the anticrossing dispersion in the main text.

[1] W.-P. Huang, Journal of the Optical Society of America A **11**, 963 (1994).

[2] Y. Tanaka, T. Asano, Y. Akahane, B.-S. Song, and S. Noda, Applied Physics Letters **82**, 1661 (2003).
